# Supplementary material for: NDJIR: Neural Direct and Joint Inverse Rendering for Geometry, Lights, and Materials of Real Object
Source: arXiv:2302.00675 source file (2023-02-02)

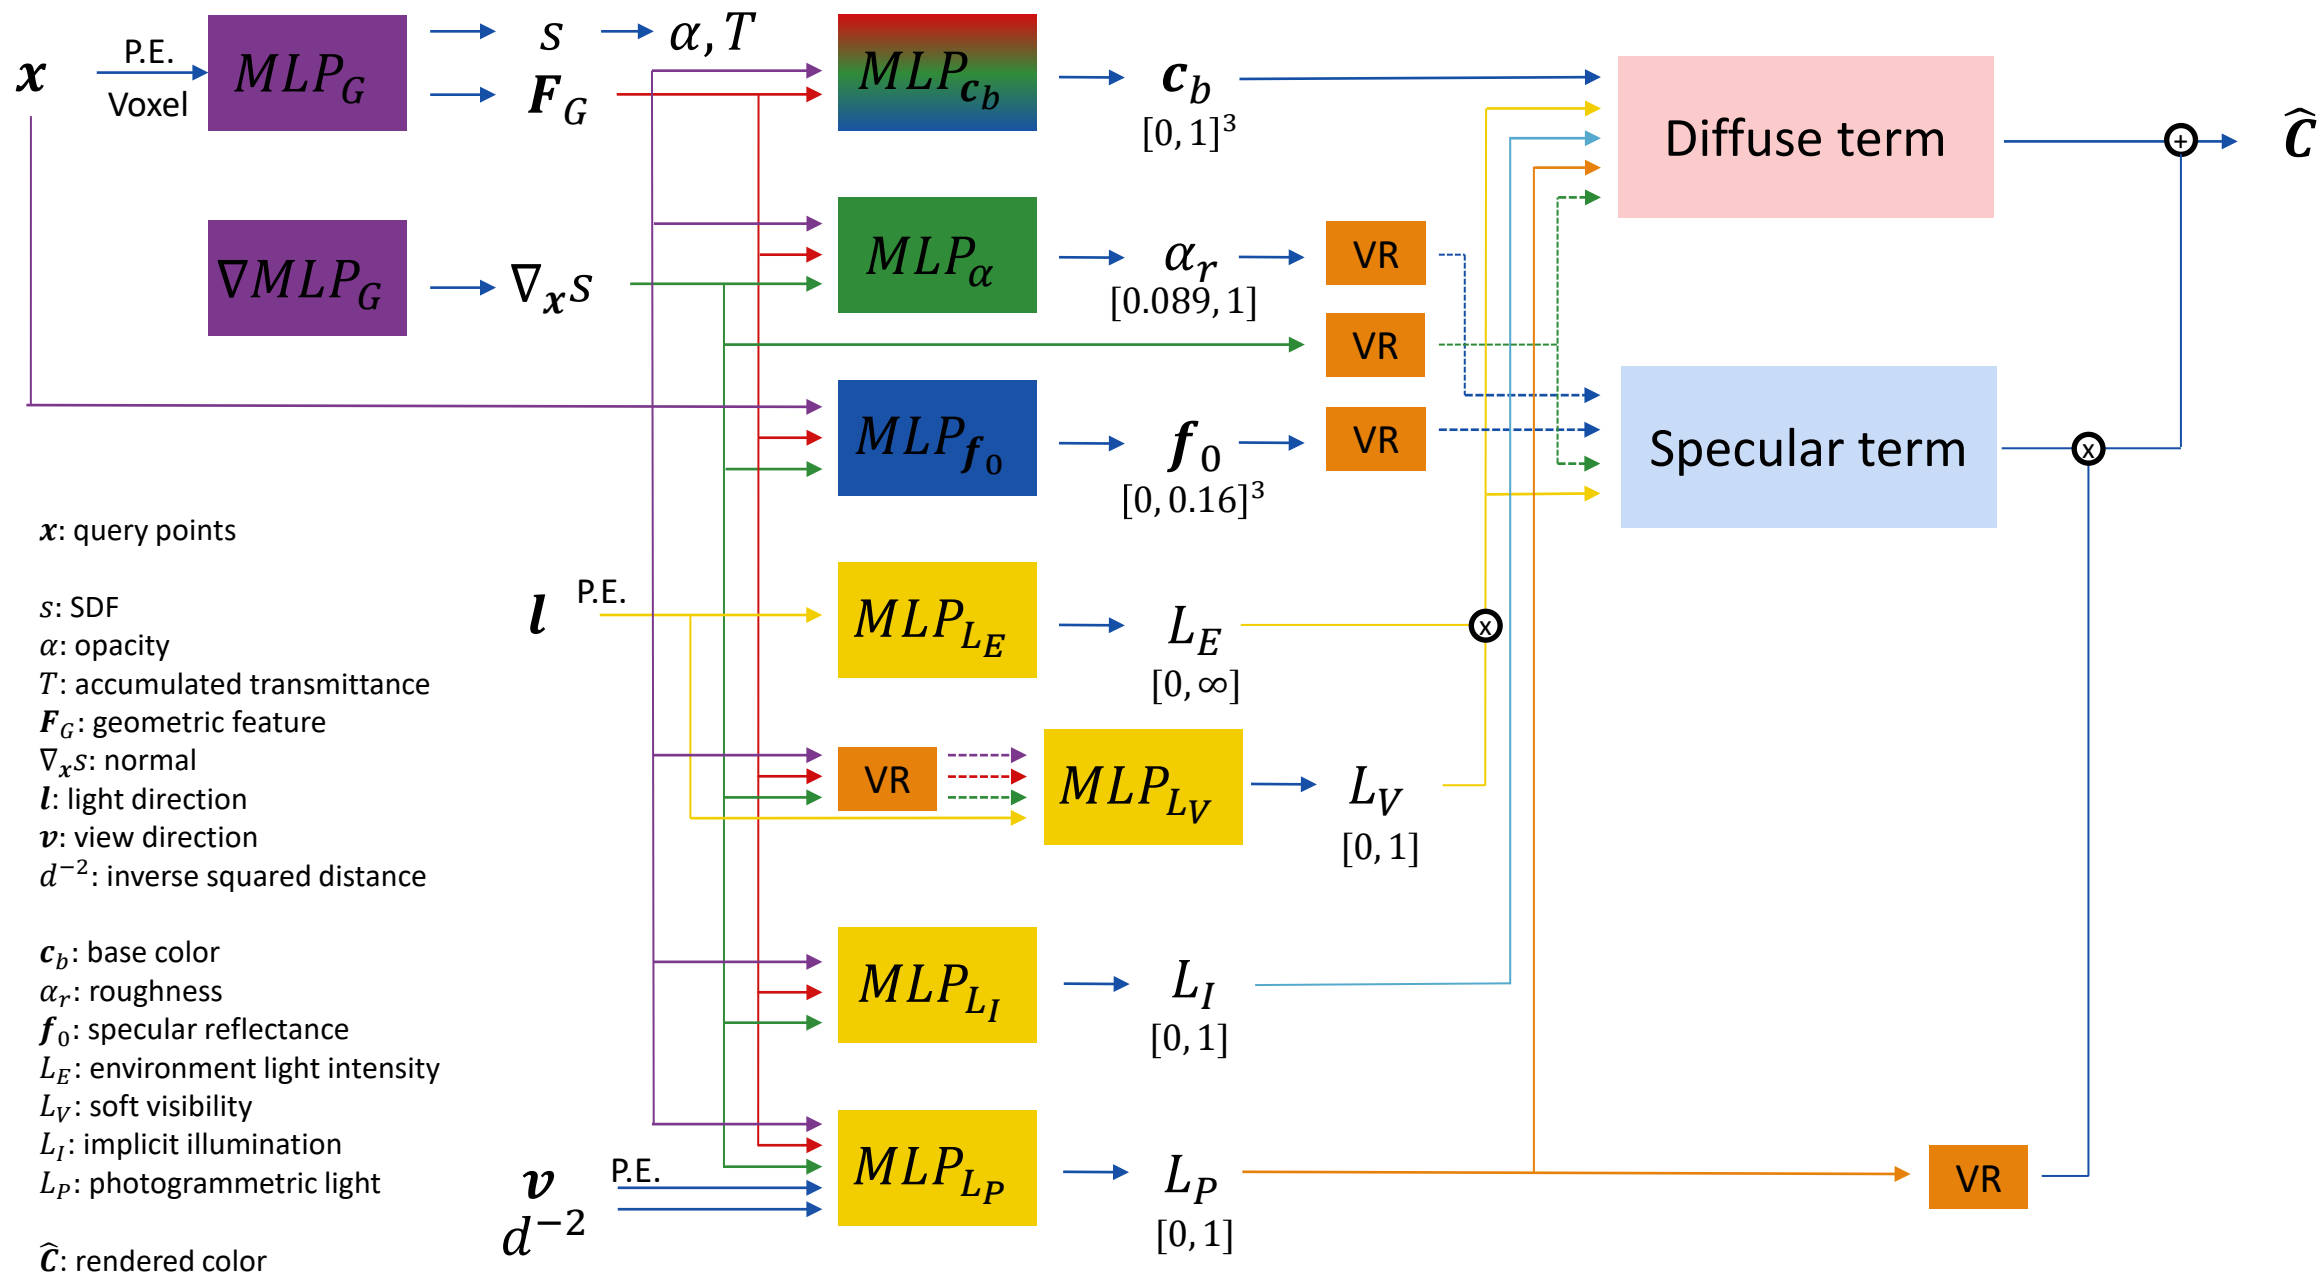

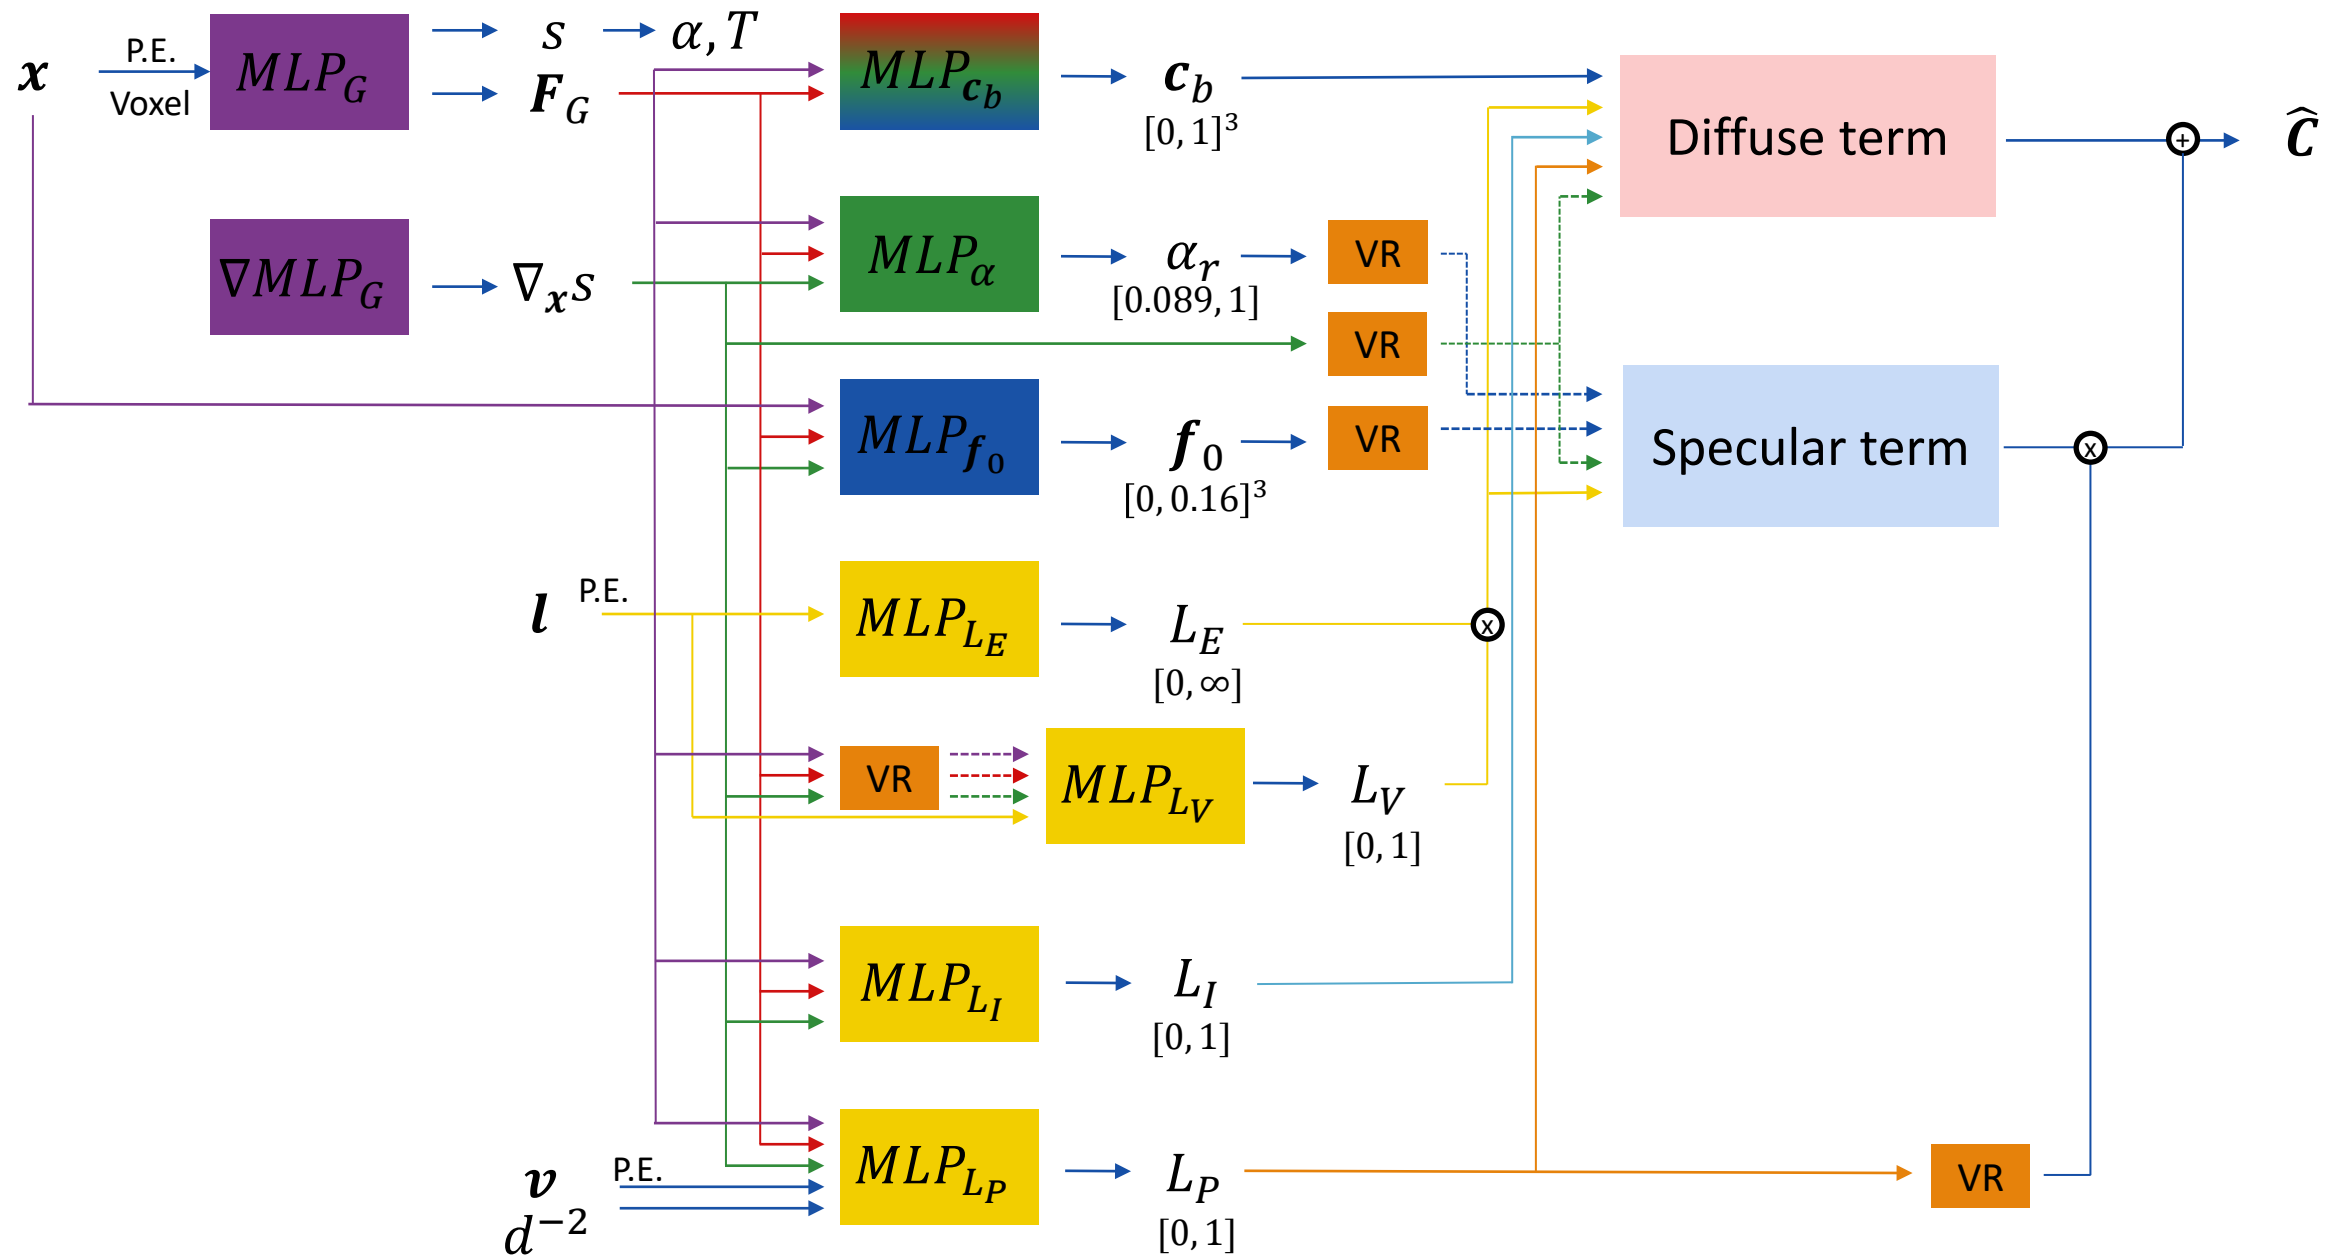

Supplement: Supplementary file 1 [file network_diagram.pdf]
